# Supplementary material for: Neural Active Structure-from-Motion in Dark and Textureless Environment
Source: arXiv:2410.15378 source file (2024-10-20)
Supplement: Supplementary file 1 [file X_suppl.tex]

\clearpage
\setcounter{page}{1}
\title{Supplementary Material for\\ Neural Active Structure-from-Motion\\ in Dark and Textureless Environment}
% TODO FINAL: Replace with your author list. 
% Include the authors' OCRID for the camera-ready version, if at all possible.
\author{Kazuto Ichimaru\inst{1,2}\orcidlink{0000-0002-5983-5972} \and
Diego Thomas\inst{1}\orcidlink{0000-0002-8525-7133} \and
Takafumi Iwaguchi\inst{1}\orcidlink{0000-0001-9811-0993} \and \\
Hiroshi Kawasaki\inst{1}\orcidlink{0000-0001-5825-6066}}

% TODO FINAL: Replace with an abbreviated list of authors.
\authorrunning{K.~Ichimaru et al.}
% First names are abbreviated in the running head.
% If there are more than two authors, 'et al.' is used.

% TODO FINAL: Replace with your institution list.
\institute{Kyushu University, Japan\\
\url{https://www.cvg.ait.kyushu-u.ac.jp/} \and
Fujitsu Defense \& National Security Limited, Japan\\
\url{https://www.fujitsu.com/jp/group/fdns/}}
\maketitle

\section{Procedure of system pose noise addition}
In this section, we explain the detailed procedure of system pose noise addition.
Assume we have ground-truth system rotation $\bm{r}_i^{gt}$ and translation $\bm{t}_i^{gt}$, which convert the camera coordinate system into the world coordinate system (\ie, $\bm{t}_i^{gt}$ are the true camera positions in world coordinate system).
To determine the scale of the scene, we compute baseline $T$, as follows:
\begin{equation}
    T = \frac{1}{N-1} \sum_{i=0}^{N-1} \left| \bm{t}_i^{gt} - \bm{t}_{i-1}^{gt} \right|_2,
\end{equation}
where $N$ is the number of the images.
Once rotational noise scale $\delta_{r}$ and translational noise scale $\delta_{t}$ are specified, we compute initial system rotation $\bm{r}_i^{init}$ and translation $\bm{t}_i^{init}$ as follows:
\begin{equation}
    \begin{split}
        r &= U(-\delta_{r} / 2, +\delta_{r} / 2), \\
        p &= U(-\delta_{r} / 2, +\delta_{r} / 2), \\
        y &= U(-\delta_{r} / 2, +\delta_{r} / 2), \\
        \bm{r}_i^{noise} &= euler(r, p, y), \\
        \bm{r}_i^{init} &= SO3(so3(\bm{r}_i^{noise}) \cdot so3(\bm{t}_i^{gt})), \\
        x &= U(-\delta_{t} / 2, +\delta_{t} / 2) \cdot T, \\
        y &= U(-\delta_{t} / 2, +\delta_{t} / 2) \cdot T, \\
        z &= U(-\delta_{t} / 2, +\delta_{t} / 2) \cdot T, \\
        \bm{t}_i^{init} &= \bm{t}_i^{gt} + (x, y, z)^T, \\
    \end{split}
\end{equation}
where $euler$ makes rotation vector from roll, pitch, yaw, $so3$ makes rotation matrix from rotation vector, $SO3$ makes rotation vector from rotation matrix, and $U(a, b)$ is uniform noise with range of $a$ to $b$.

\section{Evaluation metrics}

As mentioned in the main text, we used Chamfer distance (reconstructed shape to GT shape) to measure the accuracy of the reconstructed shapes.
However, we noticed too large values were obtained from the reconstructed shapes with many outliers, such as Light-sectioning.
Thus, we added the following pre-processes before computing Chamfer distance for fair comparison.
\begin{enumerate}
    \item Adjust rotation, translation and scale of the estimated poses to fit the GT poses to remove ambiguity on global transformation.
    \item Compute the point-to-point distances between the reconstructed shapes and the GT shapes, and remove points with minimum distance larger than 5\% of the scene boundary as outliers.
\end{enumerate}

\section{Evaluation on various pose noise scales}

In this section, we show the results of additional experiments on various range of pose noise scales in \autoref{tab:various_pose_noise} and \autoref{tab:various_pose_noise2}.
Specifically, we tried $10^\circ,20^\circ$ for rotation, and $50\%, 100\%$ for translation.

As the results show, the proposed method consistently outperforms the comparative methods.
Light-sectioning sometimes surpasses the proposed method for larger pose noises, which is because the NeRF-based methods tend to fail to converge when the scale of noise is large, which is a limitation of NeRF-based localization.
%However, the reconstructed shapes are corrupted in both light-sectioning and the proposed method, so there is little meaning in numerical comparison.

Interestingly, reconstruction accuracy is higher in no illumination with larger pose noises, despite lack of textural information.
We consider it is because textural information is beneficial only when there is enough overlap between frames, otherwise, it produces local optima.
On the other hand, the projected laser maintains a nearly constant color in the image, almost always intersecting with the other lasers in adjacent frames at some point.
This indicates new advantage of the proposed method.

\begin{table}[!ht]
    \centering
    \caption{Chamfer distances [mm] of the reconstructed shapes. Ours consistently outperforms the comparative methods. "N/A" indicates no shape reconstructed. Legend: \textbf{Best}, \underline{Second best}.}
    \label{tab:various_pose_noise}
    \scalebox{0.8}{
    \begin{tabular}{|cccc|cccc|cccc|}
    \hline
        \multirow{2}{*}{Illum} & \multirow{2}{*}{Rot[$^\circ$]} & \multirow{2}{*}{Trans[$\%$]} & \multirow{2}{*}{Method} & \multicolumn{4}{c|}{NeRF-Synthetic} & \multicolumn{4}{c|}{BlendedMVS} \\
        ~ & ~ & ~ & ~ & Lego & Chair & Hotdog & Mic & Stone & Dog & Bear & Sculpture \\ \hline
        \multirow{16}{*}{Normal} & \multirow{4}{*}{10} & \multirow{4}{*}{50} & Light-sectioning & 39.88 & 40.56 & 43.72 & 39.90 & 96.97 & \underline{25.31} & 81.32 & \underline{20.80} \\
        ~ & ~ & ~ & NeuS+Pose estim. & \underline{13.73} & 50.97 & \underline{29.10} & N/A & \underline{59.51} & 28.04 & \textbf{23.17} & 28.57 \\
        ~ & ~ & ~ & NeuS+SL & 42.59 & \underline{46.98} & 48.36 & \underline{35.13} & 85.06 & 29.80 & 46.00 & 27.64 \\
        ~ & ~ & ~ & ActiveSfM (Ours) & \textbf{13.07} & \textbf{36.93} & \textbf{22.42} & \textbf{12.13} & \textbf{31.84} & \textbf{19.89} & \underline{23.40} & \textbf{10.75} \\ \cline{2-12}
        ~ & \multirow{4}{*}{10} & \multirow{4}{*}{100} & Light-sectioning & 40.50 & \underline{37.90} & 49.99 & \underline{40.47} & 103.44 & \textbf{25.46} & 92.35 & 19.63 \\
        ~ & ~ & ~ & NeuS+Pose estim. & \underline{32.6} & N/A & \underline{48.6} & N/A & \underline{76.62} & 44.99 & \textbf{27.38} & \textbf{8.71} \\
        ~ & ~ & ~ & NeuS+SL & 41.47 & 49.33 & 51.36 & 50.34 & 90.85 & 40.74 & 55.49 & 39.04 \\
        ~ & ~ & ~ & ActiveSfM (Ours) & \textbf{25.10} & \textbf{32.59} & \textbf{44.64} & \textbf{33.66} & \textbf{40.12} & \underline{26.05} & \underline{30.85} & \underline{11.18} \\ \cline{2-12}
        ~ & \multirow{4}{*}{20} & \multirow{4}{*}{50} & Light-sectioning & 42.30 & \underline{42.80} & 50.00 & 43.93 & 93.45 & \underline{30.40} & 81.27 & 24.61 \\
        ~ & ~ & ~ & NeuS+Pose estim. & \textbf{32.6} & N/A & 48.60 & N/A & \underline{76.62} & 44.99 & \underline{27.38} & \textbf{8.71} \\
        ~ & ~ & ~ & NeuS+SL & 41.54 & 53.98 & \underline{48.15} & \textbf{36.43} & 106.52 & 35.21 & N/A & 45.85 \\
        ~ & ~ & ~ & ActiveSfM (Ours) & \underline{41.41} & \textbf{39.35} & \textbf{45.73} & \underline{40.60} & \textbf{41.02} & \textbf{28.16} & \textbf{23.63} & \underline{10.35} \\ \cline{2-12}
        ~ & \multirow{4}{*}{20} & \multirow{4}{*}{100} & Light-sectioning & 41.99 & \underline{44.81} & 48.77 & \underline{44.39} & 100.23 & \textbf{26.29} & 79.68 & \textbf{28.93} \\
        ~ & ~ & ~ & NeuS+Pose estim. & N/A & N/A & \textbf{28.84} & N/A & N/A & 39.64 & N/A & N/A \\
        ~ & ~ & ~ & NeuS+SL & \underline{40.96} & 54.74 & 55.8 & \textbf{4.15} & \underline{97.41} & 41.12 & \underline{61.98} & \underline{40.01} \\
        ~ & ~ & ~ & ActiveSfM (Ours) & \textbf{38.76} & \textbf{42.63} & \underline{46.12} & 48.78 & \textbf{39.46} & \underline{38.91} & \textbf{24.20} & N/A \\ \hline
        \multirow{16}{*}{No} & \multirow{4}{*}{10} & \multirow{4}{*}{50} & Light-sectioning & 39.88 & \underline{40.56} & \underline{43.72} & \underline{39.90} & \underline{96.97} & \underline{25.31} & \underline{81.32} & \underline{20.80} \\
        ~ & ~ & ~ & NeuS+Pose estim. & 59.75 & 48.45 & 61.15 & 43.94 & N/A & 29.31 & 81.40 & 32.26 \\
        ~ & ~ & ~ & NeuS+SL & \underline{35.04} & 44.76 & 52.76 & N/A & N/A & 50.64 & N/A & N/A \\
        ~ & ~ & ~ & ActiveSfM (Ours) & \textbf{18.50} & \textbf{18.60} & \textbf{28.47} & \textbf{6.37} & \textbf{35.36} & \textbf{21.67} & \textbf{22.99} & \textbf{11.20} \\ \cline{2-12}
        ~ & \multirow{4}{*}{10} & \multirow{4}{*}{100} & Light-sectioning & 40.05 & \textbf{37.90} & 49.99 & \underline{40.47} & \underline{103.44} & \textbf{25.46} & \underline{92.35} & \underline{19.63} \\
        ~ & ~ & ~ & NeuS+Pose estim. & 62.87 & 52.60 & \underline{45.24} & \textbf{36.50} & 112.05 & 30.29 & N/A & N/A \\
        ~ & ~ & ~ & NeuS+SL & \underline{35.04} & 44.76 & 52.76 & N/A & N/A & 50.64 & N/A & N/A \\
        ~ & ~ & ~ & ActiveSfM (Ours) & \textbf{31.26} & \underline{40.19} & \textbf{44.99} & 45.28 & \textbf{36.10} & \underline{28.57} & \textbf{22.50} & \textbf{10.68} \\ \cline{2-12}
        ~ & \multirow{4}{*}{20} & \multirow{4}{*}{50} & Light-sectioning & 42.30 & 42.80 & \underline{50.00} & 43.93 & \underline{93.45} & \textbf{30.40} & \underline{81.27} & \underline{24.61} \\
        ~ & ~ & ~ & NeuS+Pose estim. & 32.74 & 48.71 & N/A & \underline{37.67} & N/A & 49.41 & 85.97 & 27.52 \\
        ~ & ~ & ~ & NeuS+SL & \underline{28.16} & 51.67 & N/A & N/A & N/A & 43.90 & 112.48 & N/A \\
        ~ & ~ & ~ & ActiveSfM (Ours) & \textbf{18.45} & \textbf{17.64} & \textbf{28.07} & \textbf{32.84} & \textbf{36.21} & \underline{32.83} & \textbf{26.33} & \textbf{10.10} \\ \cline{2-12}
        ~ & \multirow{4}{*}{20} & \multirow{4}{*}{100} & Light-sectioning & 41.99 & \underline{44.81} & \underline{48.77} & 44.39 & \underline{100.23} & \textbf{26.29} & 79.68 & \underline{28.93} \\
        ~ & ~ & ~ & NeuS+Pose estim. & \textbf{31.70} & 54.47 & 56.56 & \textbf{22.69} & 110.47 & 48.86 & \underline{60.32} & N/A \\
        ~ & ~ & ~ & NeuS+SL & \underline{30.19} & 48.67 & N/A & N/A & N/A & 48.58 & 90.25 & N/A \\
        ~ & ~ & ~ & ActiveSfM (Ours) & 41.64 & \textbf{34.28} & \textbf{47.81} & \underline{44.06} & \textbf{38.49} & \underline{35.62} & \textbf{26.30} & \textbf{9.77} \\ \hline
    \end{tabular}}
\end{table}

\begin{table}[!ht]
    \centering
    \caption{Mean L1 errors of the estimated poses (rotation and translation). "N/A" indicates no shape reconstructed. Legend: \textbf{Best}.}
    \label{tab:various_pose_noise2}
    \scalebox{0.75}{
    \begin{tabular}{|ccccc|cccc|cccc|}
    \hline
        \multirow{2}{*}{Illum} & \multirow{2}{*}{Rot[$^\circ$]} & \multirow{2}{*}{Trans[$\%$]} & \multirow{2}{*}{Metric} & \multirow{2}{*}{Method} & \multicolumn{4}{c|}{NeRF-Synthetic} & \multicolumn{4}{c|}{BlendedMVS} \\
        ~ & ~ & ~ & ~ & ~ & Lego & Chair & Hotdog & Mic & Stone & Dog & Bear & Sculpture \\ \hline
        \multirow{16}{*}{Normal} & \multirow{4}{*}{10} & \multirow{4}{*}{50} & \multirow{2}{*}{Rot[$^\circ$]} & NeuS+Pose estim. & 0.84 & 3.90 & 1.50 & N/A & 0.60 & 3.02 & 0.96 & 2.40 \\
        ~ & ~ & ~ & ~ & ActiveSfM (Ours) & \textbf{0.56} & \textbf{1.18} & \textbf{1.29} & \textbf{0.88} & \textbf{0.52} & \textbf{0.76} & \textbf{0.38} & \textbf{0.67} \\ \cline{4-13}
        ~ & ~ & ~ & \multirow{2}{*}{Trans[$\%$]} & NeuS+Pose estim. & 4.25 & 25.63 & 9.61 & N/A & 1.37 & 7.83 & 1.53 & 4.44 \\
        ~ & ~ & ~ & ~ & ActiveSfM (Ours) & \textbf{1.43} & \textbf{7.29} & \textbf{5.59} & \textbf{3.38} & \textbf{0.09} & \textbf{0.62} & \textbf{0.43} & \textbf{0.56} \\ \cline{2-13}
        ~ & \multirow{4}{*}{10} & \multirow{4}{*}{100} & \multirow{2}{*}{Rot[$^\circ$]} & NeuS+Pose estim. & 3.82 & N/A & 3.67 & N/A & 3.74 & 4.64 & \textbf{0.85} & 2.15 \\
        ~ & ~ & ~ & ~ & ActiveSfM (Ours) & \textbf{1.95} & \textbf{1.38} & \textbf{4.04} & \textbf{3.80} & \textbf{0.79} & \textbf{3.91} & 3.98 & \textbf{0.71} \\ \cline{4-13}
        ~ & ~ & ~ & \multirow{2}{*}{Trans[$\%$]} & NeuS+Pose estim. & 28.98 & N/A & \textbf{41.24} & N/A & 7.65 & 52.78 & \textbf{4.25} & 3.64 \\
        ~ & ~ & ~ & ~ & ActiveSfM (Ours) & \textbf{14.30} & \textbf{8.13} & 44.62 & \textbf{46.59} & \textbf{0.08} & \textbf{8.16} & 5.07 & \textbf{0.70} \\ \cline{2-13}
        ~ & \multirow{4}{*}{20} & \multirow{4}{*}{50} & \multirow{2}{*}{Rot[$^\circ$]} & NeuS+Pose estim. & 7.07 & N/A & 6.08 & N/A & 4.07 & 6.83 & N/A & 8.66 \\
        ~ & ~ & ~ & ~ & ActiveSfM (Ours) & \textbf{4.91} & \textbf{4.87} & \textbf{5.37} & \textbf{7.07} & \textbf{1.03} & \textbf{3.95} & \textbf{0.42} & \textbf{1.07} \\ \cline{4-13}
        ~ & ~ & ~ & \multirow{2}{*}{Trans[$\%$]} & NeuS+Pose estim. & \textbf{25.16} & N/A & 36.99 & N/A & 4.40 & 55.78 & N/A & 15.25 \\
        ~ & ~ & ~ & ~ & ActiveSfM (Ours) & 25.36 & \textbf{25.20} & \textbf{25.14} & \textbf{25.11} & \textbf{0.09} & \textbf{4.86} & \textbf{0.39} & \textbf{1.02} \\ \cline{2-13}
        ~ & \multirow{4}{*}{20} & \multirow{4}{*}{100} & \multirow{2}{*}{Rot[$^\circ$]} & NeuS+Pose estim. & N/A & N/A & 7.42 & N/A & N/A & \textbf{7.87} & N/A & N/A \\
        ~ & ~ & ~ & ~ & ActiveSfM (Ours) & \textbf{6.27} & \textbf{7.05} & \textbf{6.01} & \textbf{6.78} & \textbf{1.26} & 7.93 & \textbf{1.71} & N/A \\ \cline{4-13}
        ~ & ~ & ~ & \multirow{2}{*}{Trans[$\%$]} & NeuS+Pose estim. & N/A & N/A & 49.1 & N/A & N/A & 20.31 & N/A & N/A \\
        ~ & ~ & ~ & ~ & ActiveSfM (Ours) & \textbf{41.2} & \textbf{43.89} & \textbf{43.37} & \textbf{48.79} & \textbf{0.07} & \textbf{13.72} & \textbf{2.07} & N/A \\ \hline
         \multirow{16}{*}{No} & \multirow{4}{*}{10} & \multirow{4}{*}{50} & \multirow{2}{*}{Rot[$^\circ$]} & NeuS+Pose estim. & 6.79 & 7.18 & 7.86 & 7.46 & N/A & 7.99 & 7.57 & 5.80 \\
        ~ & ~ & ~ & ~ & ActiveSfM (Ours) & \textbf{0.74} & \textbf{1.07} & \textbf{1.02} & \textbf{0.63} & \textbf{0.53} & \textbf{1.01} & \textbf{0.42} & \textbf{0.90} \\ \cline{4-13}
        ~ & ~ & ~ & \multirow{2}{*}{Trans[$\%$]} & NeuS+Pose estim. & 25.80 & 23.86 & 25.20 & 25.95 & N/A & 10.71 & 8.60 & 17.77 \\
        ~ & ~ & ~ & ~ & ActiveSfM (Ours) & \textbf{1.48} & \textbf{3.70} & \textbf{2.97} & \textbf{2.32} & \textbf{0.41} & \textbf{1.78} & \textbf{0.48} & \textbf{0.71} \\ \cline{2-13}
        ~ & \multirow{4}{*}{10} & \multirow{4}{*}{100} & \multirow{2}{*}{Rot[$^\circ$]} & NeuS+Pose estim. & 7.68 & 8.88 & 3.22 & 4.98 & 3.58 & 8.99 & N/A & N/A \\
        ~ & ~ & ~ & ~ & ActiveSfM (Ours) & \textbf{1.19} & \textbf{1.24} & \textbf{1.82} & \textbf{1.85} & \textbf{0.65} & \textbf{3.08} & \textbf{0.48} & \textbf{1.18} \\ \cline{4-13}
        ~ & ~ & ~ & \multirow{2}{*}{Trans[$\%$]} & NeuS+Pose estim. & 47.16 & 47.26 & 68.04 & 37.25 & 12.79 & 12.11 & N/A & N/A \\
        ~ & ~ & ~ & ~ & ActiveSfM (Ours) & \textbf{1.82} & \textbf{4.53} & \textbf{6.31} & \textbf{16.18} & \textbf{0.44} & \textbf{8.04} & \textbf{0.50} & \textbf{0.79} \\ \cline{2-13}
        ~ & \multirow{4}{*}{20} & \multirow{4}{*}{50} & \multirow{2}{*}{Rot[$^\circ$]} & NeuS+Pose estim. & \textbf{0.51} & 8.65 & N/A & 9.14 & N/A & 10.09 & 10.16 & 3.58 \\
        ~ & ~ & ~ & ~ & ActiveSfM (Ours) & 1.05 & \textbf{1.02} & \textbf{1.36} & \textbf{3.39} & \textbf{0.65} & \textbf{7.11} & \textbf{0.55} & \textbf{1.28} \\ \cline{4-13}
        ~ & ~ & ~ & \multirow{2}{*}{Trans[$\%$]} & NeuS+Pose estim. & 20.4 & 25.76 & N/A & \textbf{26.22} & N/A & 10.82 & 8.80 & 7.03 \\
        ~ & ~ & ~ & ~ & ActiveSfM (Ours) & \textbf{3.38} & \textbf{3.59} & \textbf{4.17} & 26.43 & \textbf{0.40} & \textbf{10.60} & \textbf{0.59} & \textbf{1.25} \\ \cline{2-13}
        ~ & \multirow{4}{*}{20} & \multirow{4}{*}{100} & \multirow{2}{*}{Rot[$^\circ$]} & NeuS+Pose estim. & 4.31 & 9.64 & 9.45 & 7.63 & 11.06 & 9.99 & 3.67 & N/A \\
        ~ & ~ & ~ & ~ & ActiveSfM (Ours) & \textbf{2.49} & \textbf{2.02} & \textbf{5.36} & \textbf{7.20} & \textbf{0.69} & \textbf{8.52} & \textbf{0.97} & \textbf{1.69} \\ \cline{4-13}
        ~ & ~ & ~ & \multirow{2}{*}{Trans[$\%$]} & NeuS+Pose estim. & 24.35 & 49.26 & 45.24 & \textbf{52.39} & 28.18 & \textbf{12.51} & 6.56 & N/A \\
        ~ & ~ & ~ & ~ & ActiveSfM (Ours) & \textbf{1.43} & \textbf{7.42} & \textbf{39.41} & 56.34 & \textbf{0.43} & 14.02 & \textbf{0.80} & \textbf{1.81} \\ \hline
    \end{tabular}}
\end{table}

\section{Comparison to traditional SfM, state-of-the-art Neural SDF, and 3DGS}
We conducted an additional experiment using COLMAP (SfM and MVS), Neuralangelo~\cite{neuralangelo} (state-of-the-art Neural SDF) and 3DGS~\cite{3DGS} on Lego (NeRF-Synthetic), Stone (BlendedMVS), and Real (controlled sequence) scenes.
The results still show ours is advantageous in no illumination scenes, but the comparative methods achieved remarkable accuracy in normal illumination scenes.
As for 3DGS, since it is highly sensitive to initialization, it did not converge in Stone scene (\autoref{tab:more_comparison}).

\begin{table}[]
    \centering
    \scalebox{1.0}{
    \begin{tabular}{c|c|ccc|ccc}
        \hline
         Pose & \multirow{2}{*}{Method} & \multicolumn{3}{c|}{Normal illum.} & \multicolumn{3}{c}{No illum.} \\ \cline{3-8}
         noise & & Lego & Stone & Real & Lego & Stone & Real\\ \hline \hline
         \multirow{6}{*}{No} & COLMAP & \underline{6.19} & \textbf{12.04} & \textbf{7.12} & N/A & N/A & N/A\\
         & Light-sectioning & 21.08 & \underline{17.40} & 13.33 & \underline{21.08} & \textbf{17.40} & \underline{13.33}\\
         & NeRF & 23.04 & 44.31 & 18.28 & 24.75 & 63.99 & 19.44\\
         & 3DGS & \textbf{5.50} & 132.85 & 21.66 & N/A & N/A & N/A\\
         & Neuralangelo & 16.85 & 26.15 & 12.59 & N/A & N/A & N/A\\
         & Ours & 11.62 & 30.92 & \underline{9.55} & \textbf{14.97} & \underline{35.35} & \textbf{9.39}\\ \hline
         \multirow{6}{*}{Yes} & COLMAP & \textbf{6.19} & \textbf{12.04} & \textbf{7.12} & N/A & N/A & N/A\\
         & Light-sectioning & 39.88 & 96.97 & 23.45 & \underline{39.88} & \underline{96.97} & \underline{23.45}\\
         & NeRF & 56.65 & 115.54 & 25.73 & 59.16 & 121.60 & 26.18\\
         & 3DGS & 19.65 & 105.73 & 23.40 & N/A & N/A & N/A\\
         & Neuralangelo & 48.90 & 100.18 & 30.56 & N/A & N/A & N/A\\
         & Ours & \underline{13.07} & \underline{31.84} & \underline{9.27} & \textbf{18.50} & \textbf{35.36} & \textbf{12.29}\\ \hline
    \end{tabular}}
    \caption{Comparison results of traditional SfM, SL, NeRF, 3DGS, Neuralangelo. "N/A" indicates no shape reconstructed.}
    \label{tab:more_comparison}
\end{table}

\section{Pattern sparsity and scene scale}
We conducted an additional experiment for more thorough analysis.
We changed the number of lasers and applied the proposed method to Lego and Stone scenes.
The results show the proposed method works consistently regardless of the sparsity (\autoref{tab:sparsity}).

\begin{table}[]
    \centering
    \scalebox{1.0}{
    \begin{tabular}{c|cc|cc}
        \hline
        \multirow{2}{*}{Method} & \multicolumn{2}{c|}{Normal illum.} & \multicolumn{2}{c}{No illum.} \\ \cline{2-5}
         & Lego & Stone & Lego & Stone\\ \hline\hline
        NeuS + Pose estim. & 13.73 & 59.51 & 59.75 & N/A\\
        Ours (2 lasers) & 12.96 & 30.63 & 16.91 & 38.70\\
        Ours (4 lasers) & 13.07 & 31.84 & 18.50 & 35.36\\
        Ours (6 lasers) & 12.84 & 31.68 & 17.39 & 23.61\\ \hline
    \end{tabular}}
    \caption{Results of pattern sparsity analysis. "N/A" indicates no shape reconstructed.}
    \label{tab:sparsity}
\end{table}

\section{Evaluation on projector pose refinement}

\begin{figure}[t!]
    \centering
    \includegraphics[width=1.0\linewidth]{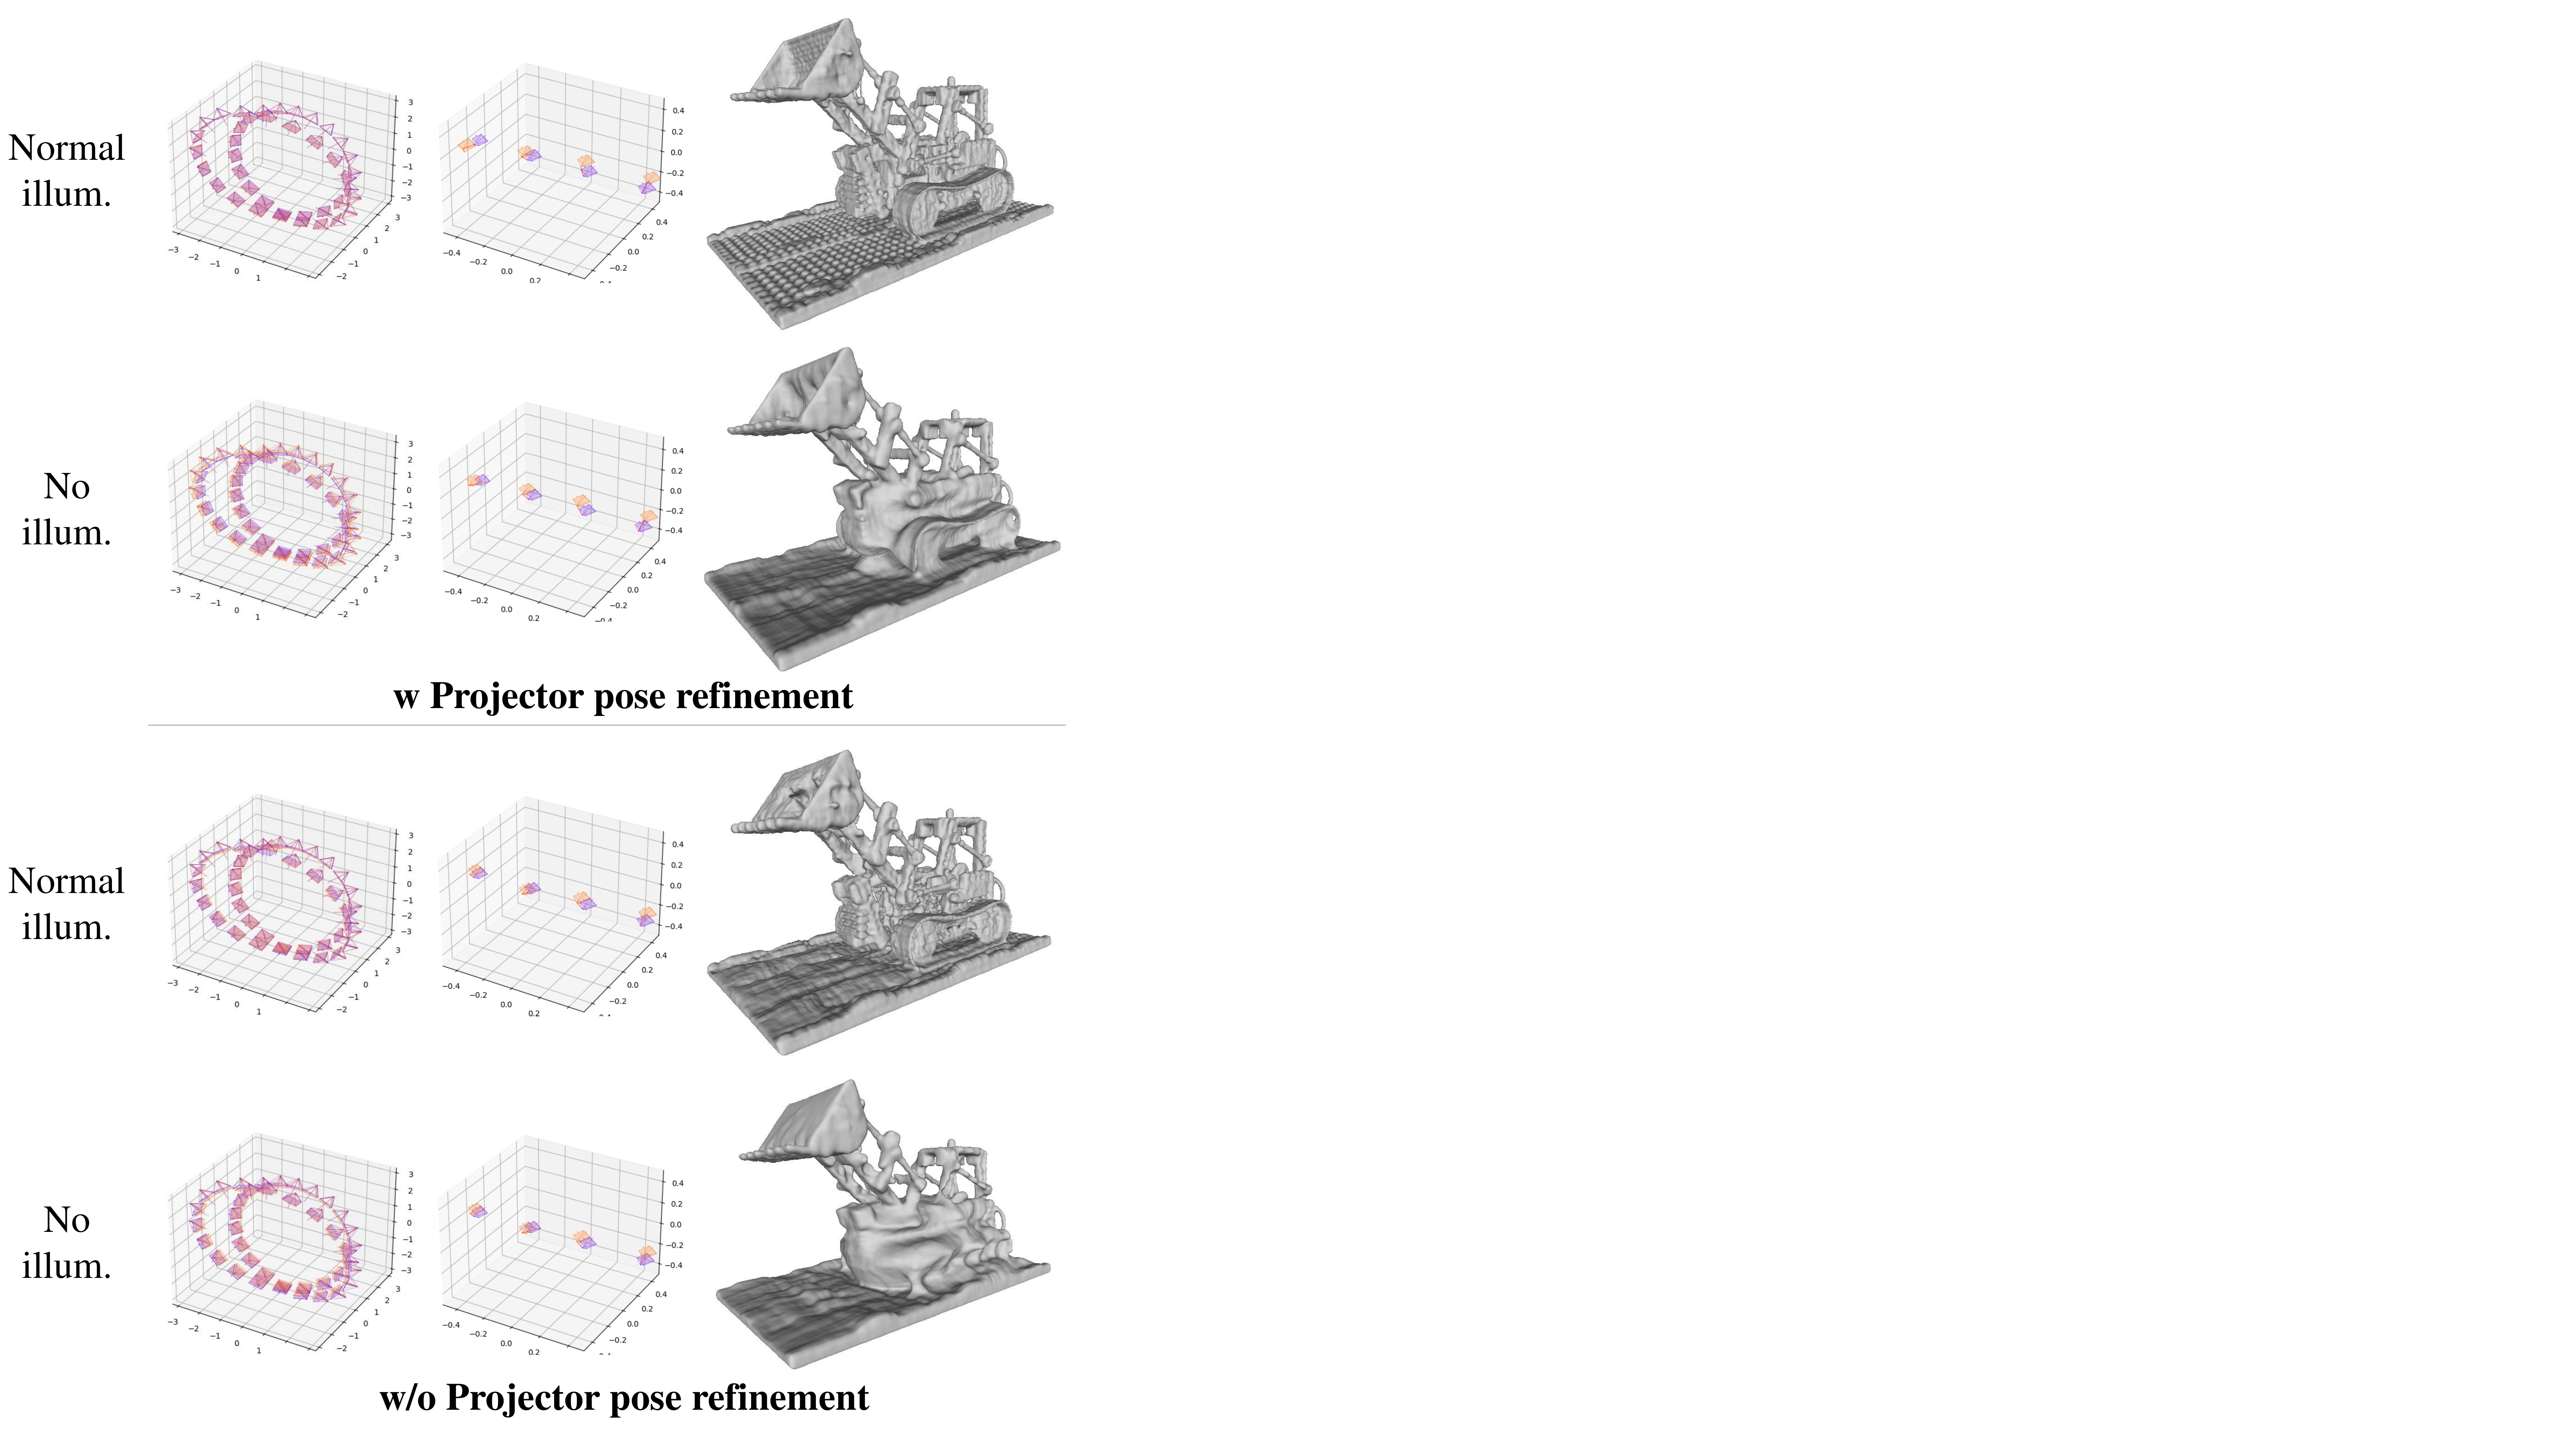}
    \caption{Qualitative results of projector pose refinement on rotational noise $4^\circ$ and translational noise $10\%$ case.
    \textbf{Left to Right}: Camera poses, projector poses, reconstructed shapes.}
    \label{fig:projector_pose_refinement}
\end{figure}

\begin{table*}[]
    \centering
    \footnotesize
    \caption{Quantitative results of evaluation on projector pose refinement. Numbers in parenthesis are the results without projector pose refinement. ``failed'' indicates they did not produce any mesh.}
    \label{tab:projector_pose_refinement}
    \begin{tabular}{|ccc|ccccc|}
        \hline
        \multirow{2}{*}{Illum} & \multicolumn{2}{c|}{Proj noise} & \multicolumn{2}{c}{Camera} & \multicolumn{2}{c}{Projector} & \multirow{2}{*}{Shape} \\
        & Rot [$^\circ$] & Trans [$\%$] & Rot [$^\circ$] & Trans [$\%$] & Rot [$^\circ$] & Trans [$\%$] & \\ \hline \hline

        \multirow{12}{*}{Normal} & \multirow{2}{*}{$0^\circ$} & \multirow{2}{*}{$5\%$} & \textbf{0.33} & \textbf{2.48} & 3.16 & 5.28 & \textbf{5.19} \\
        & & & (0.43) & (7.59) & (-) & (-) & (12.73) \\
        & \multirow{2}{*}{$0^\circ$} & \multirow{2}{*}{$10\%$} & \textbf{0.34} & \textbf{2.07} & 1.66 & 44.40 & \textbf{5.09} \\
        & & & (0.55) & (4.06) & (-) & (-) & (11.02) \\
        & \multirow{2}{*}{$2^\circ$} & \multirow{2}{*}{$5\%$} & \textbf{0.31} & \textbf{1.87} & 7.22 & 6.66 & \textbf{5.48} \\
        & & & (0.47) & (3.04) & (-) & (-) & (5.70) \\
        & \multirow{2}{*}{$2^\circ$} & \multirow{2}{*}{$10\%$} & \textbf{0.33} & \textbf{1.93} & 4.34 & 10.02 & \textbf{5.32} \\
        & & & (0.45) & (3.05) & (-) & (-) & (5.50) \\
        & \multirow{2}{*}{$4^\circ$} & \multirow{2}{*}{$5\%$} & \textbf{0.29} & \textbf{2.10} & 7.52 & 6.46 & \textbf{5.18} \\
        & & & (0.97) & (6.58) & (-) & (-) & (7.83) \\
        & \multirow{2}{*}{$4^\circ$} & \multirow{2}{*}{$10\%$} & \textbf{0.38} & \textbf{3.23} & 11.88 & 10.13 & \textbf{5.73} \\
        & & & (0.70) & (8.17) & (-) & (-) & (7.07) \\ \hline

        \multirow{12}{*}{No} & \multirow{2}{*}{$0^\circ$} & \multirow{2}{*}{$5\%$} & \textbf{0.41} & \textbf{17.43} & 0.41 & 5.40 & \textbf{14.78} \\
        & & & (0.44) & (25.80) & (-) & (-) & (18.62) \\
        & \multirow{2}{*}{$0^\circ$} & \multirow{2}{*}{$10\%$} & \textbf{0.44} & \textbf{14.05} & 0.60 & 9.79 & \textbf{11.18} \\
        & & & (0.52) & (32.11) & (-) & (-) & (19.19) \\
        & \multirow{2}{*}{$2^\circ$} & \multirow{2}{*}{$5\%$} & \textbf{0.51} & \textbf{11.50} & 4.83 & 6.80 & \textbf{9.39} \\
        & & & (5.84) & (42.12) & (-) & (-) & (failed) \\
        & \multirow{2}{*}{$2^\circ$} & \multirow{2}{*}{$10\%$} & \textbf{0.42} & \textbf{9.98} & 0.10 & 49.11 & \textbf{9.07} \\
        & & & (5.83) & (39.61) & (-) & (-) & (failed) \\
        & \multirow{2}{*}{$4^\circ$} & \multirow{2}{*}{$5\%$} & \textbf{0.54} & \textbf{9.24} & 2.96 & 6.69 & \textbf{15.34} \\
        & & & (0.65) & (11.18) & (-) & (-) & (17.20) \\
        & \multirow{2}{*}{$4^\circ$} & \multirow{2}{*}{$10\%$} & \textbf{0.43} & \textbf{7.53} & 2.69 & 10.40 & \textbf{12.44} \\
        & & & (0.67) & (9.71) & (-) & (-) & (17.48) \\

        \hline
    \end{tabular}
\end{table*}

\begin{comment}
\begin{table}[]
    \centering
    \small
    \caption{Quantitative results of evaluation on projector pose refinement.}
    \label{tab:projector_pose_refinement}
    \begin{tabular}{|cc|ccccc|}
        \hline
        \multirow{2}{*}{Illum} & Proj pose & \multicolumn{2}{c}{Camera} & \multicolumn{2}{c}{Projector} & \multirow{2}{*}{Shape} \\
        & refinement & Rot [$^\circ$] & Trans [$\%$] & Rot [$^\circ$] & Trans [$\%$] & \\ \hline \hline

        \multirow{2}{*}{Normal} & Yes & \textbf{0.38} & \textbf{3.23} & 11.88 & 10.13 & \textbf{5.73} \\
        & No & 0.70 & 8.17 & - & - & 7.07 \\ \hline

        \multirow{2}{*}{No} & Yes & \textbf{0.43} & \textbf{7.53} & 2.69 & 10.40 & \textbf{12.44} \\
        & No & 0.67 & 9.71 & - & - & 17.48 \\

        \hline
    \end{tabular}
\end{table}
\end{comment}

We also conducted another evaluation on projector pose refinement.
We empirically observed that large projector pose error leads to severe collapse of the reconstructed shapes, but small errors can be refined by defining the projector poses as learnable parameters.
Therefore, we added $0,1,4^\circ$ rotational noise and $5,10\%$ translational noise on the projector poses in addition to the camera poses with $10^\circ$ rotational noise and $50\%$ translational noise.
%Therefore, we added $4^\circ$ rotational noise and $10\%$ translational noise on the projector poses in addition to the camera poses with $10^\circ$ rotational noise and $50\%$ translational noise (Please refer to the supplementary material for further evaluation results with other noise scales).
Note that since we assume projectors are fixed relative to the camera, we have only 6 parameters to refine per projector.
To verify the effectiveness of the proposed method, we also trained the pipeline without projector pose refinement.

\autoref{fig:projector_pose_refinement} and \autoref{tab:projector_pose_refinement} shows the qualitative and quantitative results of the evaluation.
As the results show, reconstruction and pose estimation quality are consistently improved by projector pose refinement.
We noticed the projector pose estimation accuracy is considerably bad despite the drastic improvements in the reconstruction quality.
This is presumed to be because the pattern projected by the projectors was a cross-laser pattern, which left degrees of freedom in the pose of the projector, especially in the no illumination where textural information is not available.
It is rather interesting the training was performed to maintain the consistency of the scene and the reconstruction results were accurate, even in such an under-constrained problem.

\begin{comment}
\section{Results without pose estimation}
In this section, we show the reconstructed shapes without pose estimation to demonstrate small pose noise leads to severe corruption.
\autoref{fig:wo_pose_estimation} shows the whole results.
All results were obtained with $10^\circ$ rotational and $50\%$ translational noise (the easiest case).
As the results show, we could not get meaningful shapes at all; proving the importance of the proposed method.

\begin{figure}[t!]
    \centering
    \includegraphics[width=1.0\linewidth]{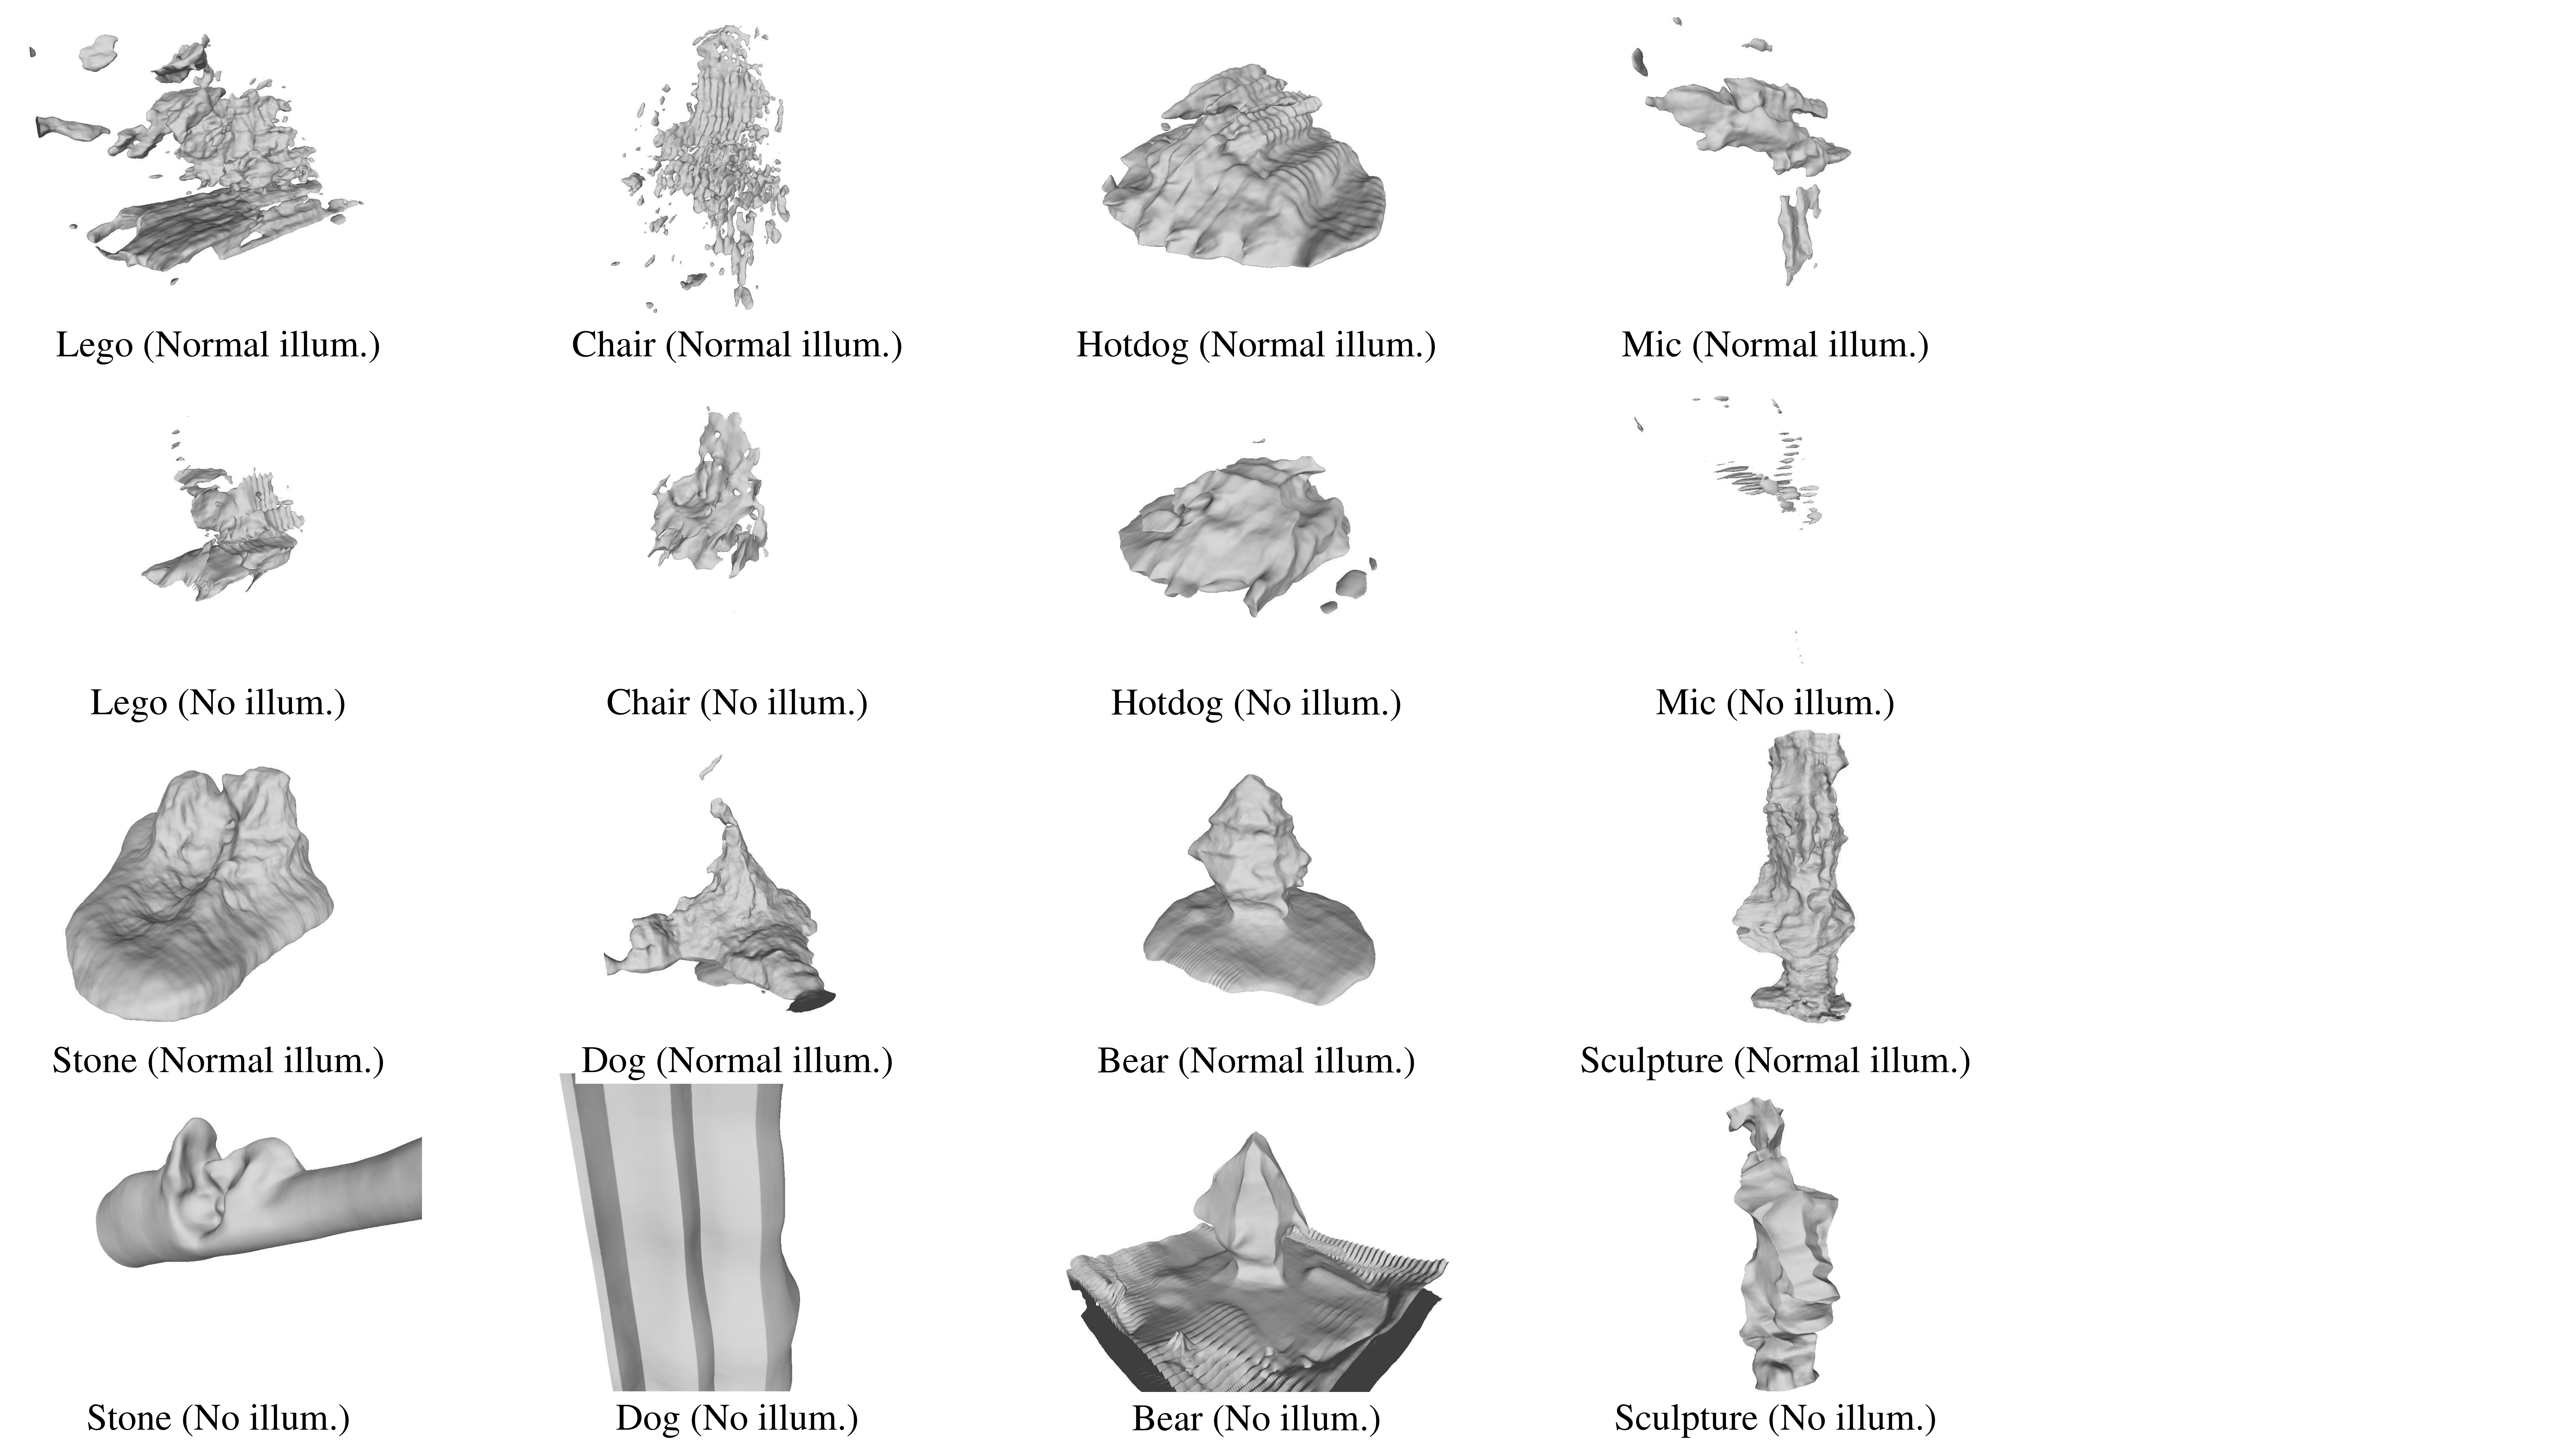}
    \caption{Reconstructed shapes without pose estimation.}
    \label{fig:wo_pose_estimation}
\end{figure}
\end{comment}

\section{Evaluation without mask loss}
During the experiments, we used mask loss to separate NeRF-Synthetic, BlendedMVS, and controlled sequence scenes.
However, some may wonder if object mask is not available in dark environments, and in that case, using mask loss does not make sense.
Therefore, we conducted another experiment to clarify how the proposed method works in the dark environment without mask loss.
Specifically, we ran evaluations on shape reconstruction accuracy and pose estimation accuracy on NeRF-Synthetic and BlendedMVS as same as the main text, but without mask loss.
\autoref{fig:wo_mask} shows the qualitative results and \autoref{tab:wo_mask} shows the quantitative results.
From the results, we can say it is possible to run ActiveSfM without mask loss, but its accuracy is suboptimal compared to that with mask loss, and enhancing the robustness is the future work.

\begin{figure}
    \centering
    \includegraphics[width=1.0\linewidth]{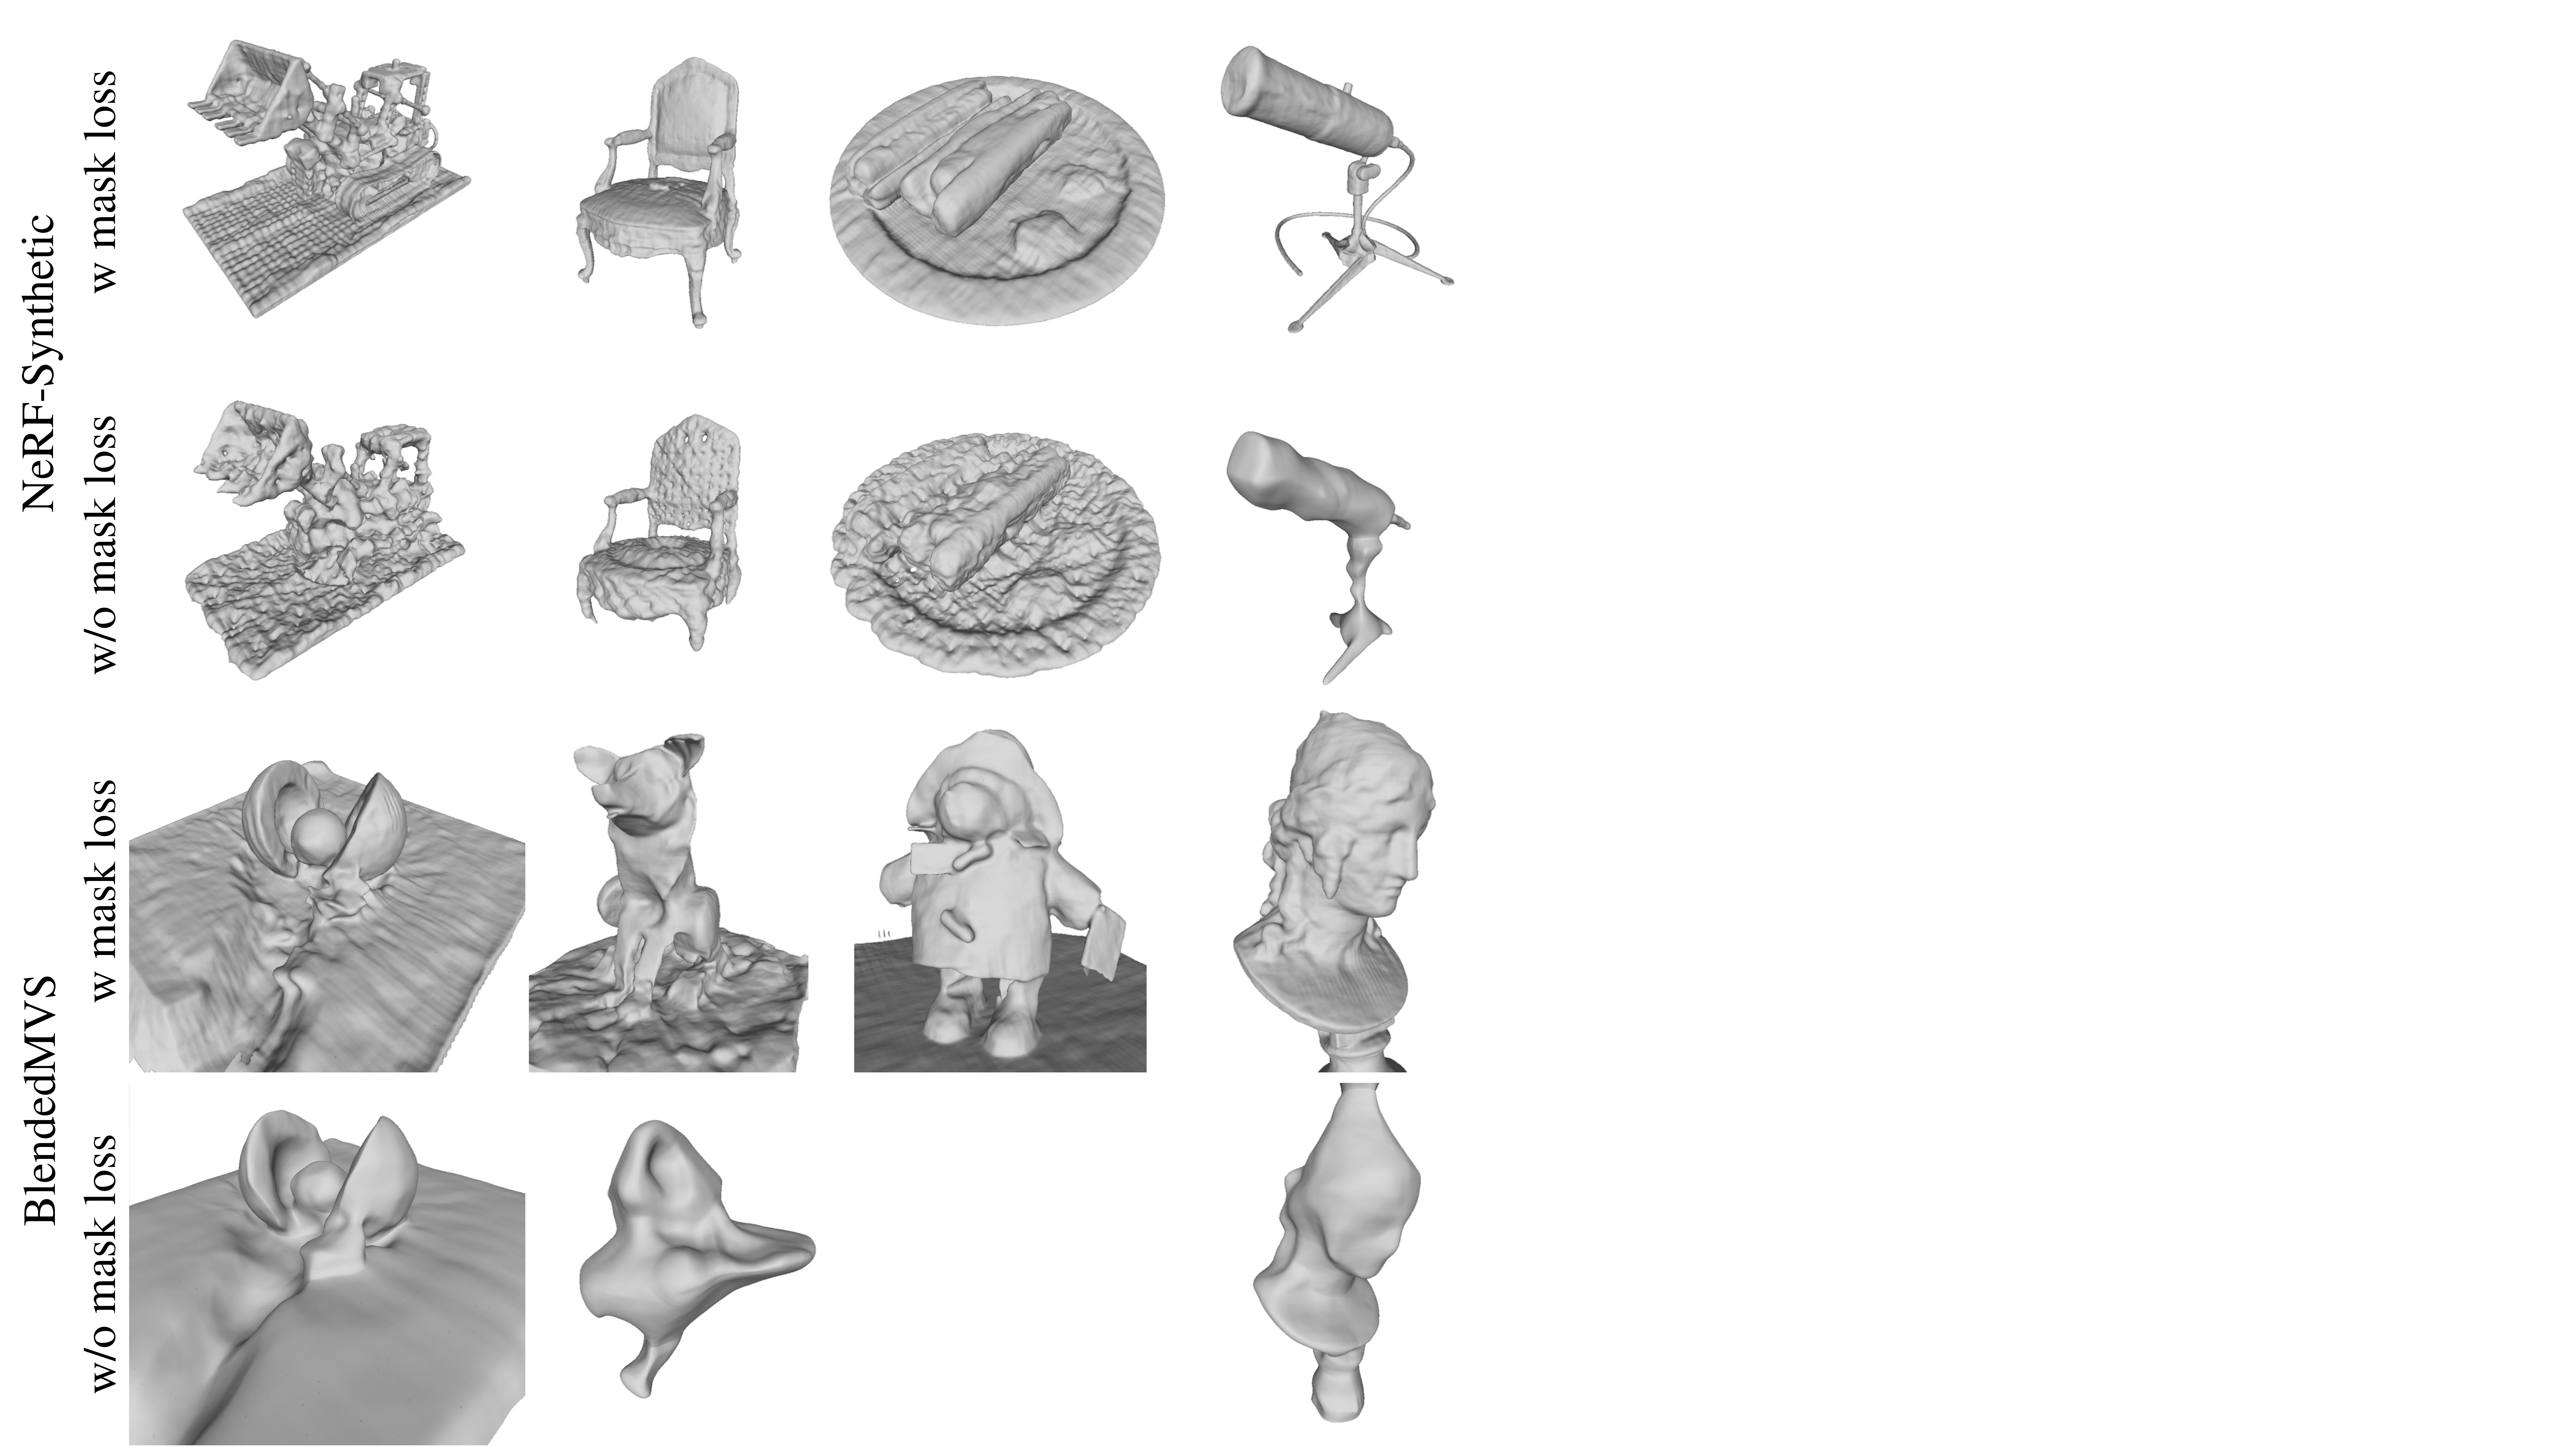}
    \caption{Qualitative comparison with and without mask loss.}
    \label{fig:wo_mask}
\end{figure}

\begin{table}[t]
    \centering
    \begin{tabular}{|c|cccc|cccc|}
    \hline
        \multirow{2}{*}{Method} & \multicolumn{4}{c|}{NeRF-Synthetic} & \multicolumn{4}{c|}{BlendedMVS} \\
         ~ & Lego & Chair & Hotdog & Mic & Stone & Dog & Bear & Sculpture \\ \hline \hline

         ActiveSfM (w mask loss) & 18.50 & 18.60 & 28.47 & 6.37 & 35.36 & 21.67 & 22.99 & 11.20 \\ \hline
         ActiveSfM (w/o mask loss) & 25.47 & 14.58 & 25.46 & 9.10 & 31.88 & 10.40 & N/A & 12.39 \\ \hline
    \end{tabular}
    \caption{Quantitative comparison in Chamfer distance (mm) with and without mask loss. N/A indicates no shape reconstructed.}
    \label{tab:wo_mask}
\end{table}

\section{Details of the experimental system configuration}
In \autoref{tab:system_configuration}, we briefly explain the details of the experimental system configuration used in \autoref{sec:experiments}.
As for the devices, we used a Basler camera and commercial cross laser projectors.

\begin{table}[t!]
    \centering
    \begin{tabular}{|c|c|}
        \hline
        \multirow{3}{*}{Image resolution} & 800x800 (NeRF-Synthetic) \\
        & 768x586 (BlendedMVS) \\
        & 1280x960 (Real) \\ \hline
        Laser wavelength & $520 \pm 10 nm$ \\ \hline
        Line thickness & 3mm at 1m away \\ \hline
    \end{tabular}
    \caption{Details of the experimental system configuration.}
    \label{tab:system_configuration}
\end{table}

\section{Procedure of synthetic image generation}
Here, we explain the procedure of the synthetic image generation used in \autoref{ssec:synthetic_evaluation}.
Assume we have the original images $J(\bm{p})$ and GT depth images $D(\bm{p})$.
For each 2D point $\bm{p}$, we back-project it to the world coordinate system to obtain 3D point $\bm{P}_s$ as follows,
\begin{equation}
    \bm{P}_s = \bm{R}_i \cdot K_c^{-1} \bm{p}^T D(\bm{p}) + \bm{t}_i, \\
\end{equation}
then, re-project it to the $k$-th projector screen coordinate system to obtain the projected color onto the point $\bm{P}_s$,
\begin{equation}
    Q_k(\bm{P}_s) = I^k(K^k(R^k\bm{P}_s + \bm{t}^k)^T),
\end{equation}
finally, pixel color of the synthesized image $J'$ on $\bm{p}$ is computed as follows,
\begin{equation}
    J'(\bm{p}) = J(\bm{p}) + \sum_{k=1}^{N_p} o(\bm{P}_s, k) (i_{r}^{GT}J(\bm{p}) + i_{b}^{GT})Q_k(\bm{P}_s),
    \label{eq:color_blend}
\end{equation}
where $i_r^{GT}$ and $i_b^{GT}$ are GT illumination parameters, and $o(\bm{P}_s, k)$ returns $1$ if $\bm{P}_s$ is not occluded by other points when viewed from the $k$-th projector, otherwise returns $0$.
Occlusion is computed using Z-buffer in our implementation.

\section{Procedure of dark image synthesis}
As for the dark image synthesis used in \autoref{ssec:real_evaluation}, we simply scaled the intensities of the images to simulate quantization error in 8-bit image format.
Other types of noise are the future work, like high ISO noise or motion blur.

\section{On GNSS \& IMU accuracy}
Some people may have a doubt if GNSS or IMU accuracy is really insufficient for 3D measurement.
The accuracy of common GPS is said to be 1-3 meters, and that of common IMU is said to be 2-5 centimeters and 0.005-0.015 degrees, which are covered in the experiments.
This may be acceptable for large scale capturing, while it may be impossible to recover a meaningful trajectory in micro-baseline settings.
Our structured light system is intended for the latter use-cases, such as underwater facility inspection or endoscopic surgery.

\section{Implementation details of comparative methods}
In general, we used official implementations for the comparative methods in the experiments.
However, we had to modify a little bit to acquire the results, which is described below.

\paragraph{Light-sectioning}
Light-sectioning is a general principle for 3D shape reconstruction with active projection, and there are no specific implementation.
Therefore, we implemented light-sectioning by ourselves from scratch.

\paragraph{LLNeRF~\cite{llnerf}}
Since the official implementation does not provide a feature for mesh reconstruction, we implemented mesh reconstruction feature by marching cubes with the obtained density values from MLP.
As for the hypermarameter, we does not change them except near / far clip and data loss function.
Because the original rawnerf loss function did not converge well with our data, we replaced it with Mean-Squared-Error (mse).

\paragraph{NeuS~\cite{NeuS}}
We used the official implementation with few modifications.
Specifically, we increased resolution for mesh reconstruction to obtain finer results and re-implemented camera parameters as learnable parameters for NeuS+Pose estimation.
Note, NeuS does not update camera parameters by itself (no gradients are computed).

\paragraph{NeuS+Pose estimation}
We added the pose estimation pipeline identical to ours on NeuS.
We can also say it is SDF-based NeRF--~\cite{NeRF--}.

\paragraph{NeuS+SL}
NeuS+SL is identical to the proposed method without pose estimation, as mentioned in the main text.
